# Supplementary material for: Wikipedia and Westminster: Quality and Dynamics of Wikipedia Pages about UK Politicians
Source: arXiv:2006.13400 source file (2020-06-24)
Supplement: Supplementary file 1 [file appendix.tex]

\subsection{introduction}
Understanding collective attention on MP pages is crucial to quantify both the exposure of citizens to political Wikipedia content, and the extent of the collaborative efforts supporting the evolution of the articles. To shed light on these dynamics, we first investigate how attention load on MP pages (both in terms of edits and views)  shifts during  ``times of shock", and look at the temporal and spatial distribution of contributions to those Wikipedia articles.

\subsection{Related work}

MPs consider and propose new laws. They can scrutinise government policies by asking government ministers questions about current issues in the Commons Chamber, in Committees or in writing.

\textbf{Readers' Engagement with Wikipedia}
Many studies focus on quantifying and qualifying different forms of readers engagement on Wikipedia pages. A reading behavior study based on a survey by Singer et al ~\cite{singer2017we} identified a set of reasons why readers go to Wikipedia. These motivations include: reading about a recent event, personal interest, work or study, and boredom.   

A recent work~\cite{zhang2019participation} finds that during ``shock periods'' there is a significant increase in new editors. These new users find it hard to participate at first and their edits are mostly reverted by regular editors. 
In controversial pages, usual editing patterns involve a phenomenon which is known as ``edit wars''~\cite{yasseri2012dynamics} where volunteers try to add and revert contributions in a short span of time. 
Editors are especially active during election times~\cite{keegan2019dynamics, gobel2018political, neff2013jointly}, for example pages of Donald Trump and Hillary Clinton were heavily modified during the 2016 US Presidential campaign~\cite{keegan2019dynamics}.

Recent studies~\cite{asthana2018few,ores} proposed automatic review methods for new articles and new edits. Using automatic topic models, improper edits which are often overlooked during the manual review process can be identified. The ORES ~\cite{ores} tool uses such models to maintain quality of edits and articles by classifying them at scale.

\subsection{dataset}
We collect party labels including Conservative (318), Labour (262), Scottish National (or SNP, 35) and others (35), and gender labels: male (442) and female (208) for each MP. 
We verify our dataset with the UK Parliament's 2017 general election dataset and analysis~\cite{ukelectionStats2017}.
Note that we also verify from the official record that all 650 MPs are either male or female\footnote{\url{pinknews.co.uk/2019/12/13/powerful-transgender-lobby-0-openly-trans-non-binary-mps/},Accessed 26 Feb 2020}. 
Each position held entry has extensive details such as start date, end date, name of the politician replaced, etc. We find that an MP holds 3--4 (median 3) positions during a political career with a maximum of 14 for the MP \emph{Kenneth Clarke} since 1970.

\subsection{dynamics}

%In this section we investigate spatio-temporal interactions with MPs' Wikipedia pages.% by looking the spatio-temporal  of pages. 
%\pushkal{Improve skeleton here to connect the different subsections.}
\subsubsection{Page Creation}
%To understand the information broadcast via MPs pages 
%We first investigate characteristics of creation of UK MP pages.  %\footnote{Between the launch of Wikipedia on January 15, 2001 and September 2007 there are two million English language articles.}
%This is likely to be the rapid growth of Wikipedia itself during 2002 to 2004.

To understand better if the creation of a Wikipedia page for an MP correlates to the MP's first position (as an MP) in the Parliament, we make use of \emph{Position held} data available in Wikidata (discussed in \S~\ref{sec:dataset}). We eliminate from consideration those MPs who first held their post before the Wikipedia was born and take the remaining 488 (75\%) MPs from the 2017 Parliament who were elected for the first time during 2005, 2010, 2015 or 2017 general elections. We compare the year of their first election to the corresponding Wikipedia page creation year. In Figure~\ref{fig:pageYear}  shows the number of MPs' pages created each year, as well as the number of MPs holding their first position as MPs each year. Interestingly, we see that almost 77\% of MPs pages were created in the year they were first elected (Pearson's correlation between page creation and first position held is 80\% ($p<0.001$)).  \textit{In other words, MP pages are created soon after MPs are elected, except for the minority of MPs who have held their seats from before the Wikipedia was born.}
%To calculate the similarity of these two distributions, we compute the KL (Kullback-Leibler) Divergence~\cite{kullback1951information}

By checking day-by-day records, we see that for 26\% of MP pages their creation dates are same as their first position date. Moreover, page creations for 20\% of MPs are one-day after, 2\% one-day before and 2\% for two to thirty days before the MPs' first position held date. In total, 72\% (28\%) of pages are created on or after (just before) the date of their election. In party-wise breakdown we see that unlike Conservative (72\%) and Labour (73\%) party pages, a very high proportion (88\%) of SNP pages are created after their election. For MPs of other parties, this proportion is as low as 42\%.

\subsection{polarisation}

Next, we look at the distribution of edits by editors labeled with different political leanings. In Figure~\ref{fig:crossPartyHeat} we show on the x-axis MPs' parties and on the y-axis editors' parties. Each cell shows, for a given party the fraction of edits by editors of a party $y$ on pages of MPs with a party $x$.
The general trend in the diagonal shows that most edits are by editors identified with the same party as MPs edited. Only a minority of editors edit articles for multiple parties. For Conservative (Labour) editors 29\% (30\%) of edits are to Labour (Conservative) MPs' pages respectively. 
We also see in Figure~\ref{fig:crossPartyHeat} that for parties other than Conservative and Labour, the contributions are more partisan but almost 25\% of edits are to either Conservative or Labour Party MP pages.

\subsection{Quality of Wikipedia}
% \label{sec:quality}
%Taking the word count for each MP page we find that the mean is 1051, median is 736 and highest is 13k for MP and former Labour party leader \emph{Jeremy Corbyn}, showing that MP pages vary significantly in length.\pushkal{This section can be written as a fusion of dynamics and polarisation that relates to good quality pages. For example high viewed pages are good? Polarised groups edit better? etc.} 
We now move to analyze the quality of MPs' Wikipedia pages. We start by analyzing the quality of content which editors add. We operationalize the notion of quality through existing measures of article quality, citation quality and text readability% to develop an overall measure of quality
. First, we make use of the ORES Wikimedia API~\cite{ores} to obtain, for each article, a quality score, similar to~\cite{Redi:2019:CNT:3308558.3313618}. For citation quality, we check if a statement needs a citation and if it has a citation or not using the test developed by~\cite{Redi:2019:CNT:3308558.3313618}. Finally, we compute articles' readability using Flesch-Kincaid~\cite{si2001statistical} and other readability scores.
We provide a detailed explanation of the models used and the quality analysis result in the following subsections.

%Using a single figure star for all 3 quality plots
\begin{figure*}[thb]
    \centering
    \subfloat[Citation Quality] {
        \includegraphics[width=0.33\textwidth]{figures/missingCitationBar.png}
        %\label{fig:citation}
    }
    \subfloat[Readability] {
        \includegraphics[width=0.33\textwidth]{figures/readingPartyMain.png}
   %     \label{fig:reading}
    }
    \subfloat[Article Quality] {
        \includegraphics[width=0.33\textwidth]{figures/qualityPrediction.png}
    %    \label{fig:quality}
    }
    \caption{Dimension of pages quality. (a) Percentage of sentences which miss citation. (b) Reading Grade (RG) of main and page content per party. (c) Prediction of quality category. Darker the shade better is the page quality.}
    \vspace{-0.5cm}
\end{figure*}

\subsubsection{Categories and Section}
%The most frequently seen section headings are in Figure~\ref{fig:sectionTop}. 
There are in total 11.5k sections on the 650 MP pages, with an average of 4 sections per MP articles (up to 14 for more popular MPs). %We find a total of 392 unique section titles and on average (as well as median) there are 4 sections which can be up to 14 for more popular MPs. 
To assist our analysis of article quality, we manually group the 392 unique section titles into 12 labels% in two iterations
, avoiding overlaps in the content covered by different labels as far as possible. The label with the highest percentage of words in relation to overall article length is \emph{Political and Parliamentary career} (56\%) which includes section headings such as Parliamentary career, Member of Parliament, House of Commons etc. Next we have \emph{Early life and career} (18\%) which includes section headings such as History, Education, Background, Early Career, etc. Other major labels are Main section (10\%), Personal life (6\%), Political views (5\%) and the rest cover the remaining 5\%. 

To explore potential content biases, we breakdown section statistics party. %To understand whether at section level, take MPs' party and gender and ask if contributions to sections vary in size across these two categories.
We compute the number of words for each section label, and aggregate over all articles of MPs of specific party (for example, we take the average number of words in Main Section of Conservatives and compare with the Main section of labour MPs, etc). %\pushkal{Paragraph updated. Need to add text based on Edward's comment here. EW: paragraph updated, let me know if i've got it right!}.
To check significant differences in word count we perform the ANOVA test
%\footnote{\url{www.sthda.com/english/wiki/one-way-anova-test-in-r}}
on the resulting label distributions. %ased on average number of words for each category for each label type (for example, taking the average number of words in Main Section of Con:female, Lab:Female MPs, etc). 
We get significant differences across categories for each of the three main labels -- Political and Parliamentary career ($p<0.001$), Early Life and Career ($p<0.05$) and Main Section ($p<0.001$). The distribution between political career and early life is different for each of the three main parties. In particular Conservative MPs' pages have slightly more about political career and less about early life as compared to Labour MPs. 
%For Conservative, female MPs' pages have more about political career and less about early life than male MPs, whereas for Labour MPs, the distribution is similar for both male and female MPs. %For Labour, female MPs have more about political career, but less about early life than male MPs.
%\pushkal{Removing plot of categories and section stacked bar. This is covered in text.}

% We see from Figure~\ref{fig:partyGenderReference} that for SNP MPs, the main section comprises a larger fraction of the page. This is indicative of the rest of the page containing less detailed information in other categories such as political views and (in the case of female SNP MPs) political career. %We next see female MPs from SNP and others have less proportion of Political and Parliamentary career. A possible reason could be that female MPs are represented more in the Parliament in recent year elections than previously and hence have less records\footnote{\url{en.wikipedia.org/wiki/Women_in_the_House_of_Commons_of_the_United_Kingdom}, Accessed on 16 March 2020}. \pushkal{We need to add more details from new figure now.} 

% \begin{figure}
% \centering
% %\includegraphics[width=\columnwidth]{figures/sectionPartyWordsBar.png}
% \includegraphics[width=\columnwidth]{figures/sectionPartyWordsBar12Cat.png}
% \caption{Stacked Bar plot of words count in section for each party and gender pair.
% }~\label{fig:partyGenderReference}
% \vspace{-0.5cm}

% \end{figure}

\subsubsection{Readability}
%One way of specialisation can be a writing style. 
The next dimension of quality we analyze is readability of articles. We compute this as reading grade of the article's body, and its main section.
%As expected, we find that the main section  is easier to read than the article's body. We find that median Flesh \miriam{How does this compare to the rest of the Wikipedia?}
We use a method similar to ~\cite{brezar2019readability} to compute Reading Grade ($RG$) which is the near equivalent of reading age. This involves computing the average of 
Flesch--Kincaid ($FK$),  Simple Measure of Gobbledygook ($SMOG$) and Gunning Frequency of Gobbledygook ($FOG$) scores.~\cite{si2001statistical,benoit2018quanteda} We compute these after removing links, punctuation (except `.' and `,') and references to citations using R package~\cite{benoit2018quanteda}. We formally define Reading Grade ($RG$) as follows:

\begin{equation}
 RG=\frac{FK+SMOG+FOG}{3}
\end{equation}
%\ns{is this your definition? If so, why is taking a mean of the three scores useful? And are they all on the same scale from 0-100? If not you cannot just merge them in a linear fashion. }\pushkal{We use this formula from~\cite{brezar2019readability} as stated above.}
We plot $RG$ of main section and page content of each MP page in Figure~\ref{fig:reading}. We see that main sections (median $RG=15.55$) are easier to read than page content ($RG=18.15$). In~\cite{brezar2019readability}, the authors report that the average $RG$ of the twenty-five most-viewed Wikipedia pages on diseases is 12.73 (sd: 0.32). This shows that over the years disease pages become easy to read with high and significant correlation between $FK$, $SMOG$ and $FOG$. They categorise $RG$ scores as under 12--fairly difficult (High school), 12 to 14--difficult (College level) and above 14--very difficult (College graduate level). We check percentage of main section and page content of MP articles based on this categorisation. We find that the main section of 9\% of pages are fairly difficult, 21\% are difficult and 70\% are very difficult. For overall page content 0.6\% of pages are fairly difficult, 1\% are difficult and the rest 98\% are very difficult. %\pushkal{Are we interested in knowing what are these difficult sections of the page content? EW: It would be more interesting to know why the pages are so difficult, but that will have to wait for another paper!}

We also break down the $RG$ score by party, and find that Labour and SNP pages are easier to read than Conservative (KS-stats: (Con, Lab) D=0.16 and p<0.001, (Con, SNP) D=0.34, p<0.001). We show per party distribution in Figure~\ref{fig:reading}.%\pushkal{These numbers are distance in the distribution and if that if significant or not.}

\subsection{Article Quality}
The ORES~\cite{ores} API computes the probability of an article belonging to a given quality category  based on page length, infobox, number of images, sections etc. Given an article, ORES returns 6 probability scores, one for each quality level (\textit{Start, Stub, C-level (C), B-level (B), Good Article (GA), Featured Article (FA)})\footnote{More info- \url{en.wikipedia.org/wiki/Wikipedia:Content_assessment\#Grades}}.

In Figure~\ref{fig:quality} we show the average quality score for each quality category, broken down by MPs' parties. %(known as \emph{articlequality}) which we use from Wikimedia API  which is a \emph{drafttopic} classifier~\cite{  asthana2018few,Redi:2019:CNT:3308558.3313618}. Similar to~\cite{halfaker2017interpolating, Redi:2019:CNT:3308558.3313618} we use ORES's \emph{articlequality} model which predict level of quality of an article
%In Figure~\ref{fig:quality} we shows the predicted category based on eight quality categories provided by ORES. 
Darker shades correspond to better page quality labels.
We observe two major trends. First, despite the high overall citation quality, the quality of articles is largely poor: the majority of the articles for all parties are marked as ``C-level'', namely articles which are substantial but are  ``still missing important content or may still have significant problems which require substantial cleanup''.
Second, we observe that articles on Conservative MPs tend to be of overall higher quality. To test if this is statistically significant %Additionally 
we perform the ANOVA test, by converting quality category labels to numerical values such that 0 is Stub and 5 is Feature Article.  We find that there is a significant difference ($p<0.001$) in the ratings of articles across parties.

\subsection{survey}

We design a survey to understand the motivation of reading UK MPs' Wikipedia pages. The survey we create is a Google form questioner which we post on 6 Feb 2020 and collect 57 responses\footnote{Obtained approval from our university's IRB to collect and store responses.} over a month. We discuss design and results of our survey in the following sub-sections.

\subsection{Survey design}

%https://www.ncbi.nlm.nih.gov/pmc/articles/PMC5464762/

%https://www.ifla.org/files/assets/services-for-parliaments/publications/ethics\_checklists\_preconference\_version\_20190531.pdf

The survey consists of two sections. The first records demographics and the second questions participants about their use of Wikipedia. Wherever possible we make use of similar questions from previous studies~\cite{singer2017we}. In section one we ask for three basic demographic details to establish if participants are resident/citizens of the UK, education level and age group. We give an option of `Prefer not to say'. We do not ask for any personal details such as name, gender, email, contact number etc. In section two, we ask specific questions that are constructs from the research questions we have discussed so far. Prior to sending the survey to a general audience we use a free text answer approach for some questions, asking co-authors and friends questions such as \emph{How often do you visit Wikipedia?} and \emph{Which part of MPs' Wikipedia page you think is more important to you?} Based on a handful of free text answers we add options (single or multiple choice) to make the survey easier for participants and to simplify our analysis. We also leave an option where participants can (if they wish) add a new choice. Section two of the survey can be further broken down into two sub-sections: (a) Questions related to spatio-temporal patterns (RQ1) and (b) Content quality of pages (RQ3). Note that we do not cover RQ2 in the survey as currently there is no direct way to reach editors of politicians' pages. 
%We wish to include this in our future work.
% A possible way of doing this could be showing links to a survey on editors' community (talk) pages and other platform-based approaches such as for readers\footnote{\url{meta.wikimedia.org/wiki/Research:Characterizing_Wikipedia_Reader_Behaviour/Demographics_and_Wikipedia_use_cases\#English-language_demographics_survey_questions}, Accessed 10 Feb 2020} and citations clicks.\footnote{\url{meta.wikimedia.org/wiki/Research:The\_role_of_citations_in_how_readers_evaluate_Wikipedia_articles/Surveys}, Accessed 10 Feb 2020} Nevertheless, our survey questions can be replicated to understand editors' interest while editing MPs' pages.
We present our results from the survey in the next sub-section.
% \url{https://www.ifla.org/files/assets/services-for-parliaments/publications/ethics_checklists_preconference_version_20190531.pdf}

\subsection{Survey results}

We publish our survey on many platforms (mostly in the UK) including Twitter, email groups, and direct messages. From the 57 responses, the demographics section tells us that we covered a wide spectrum of participants, mainly from the UK (86\%). Participants have education level up to high school diploma (11\%), bachelors (33\%), masters (25\%) and doctoral degree (31\%). Age group consists of categories such as 0-24 years (28\%), 25-44 years (51\%), 45-65 years (21\%) and 65-above (0\%).% No participants make use of the `prefer not to say' option.
Compared to the population Wikipedia readers\footnote{\url{https://meta.wikimedia.org/wiki/Research:Characterizing_Wikipedia_Reader_Behaviour/Demographics_and_Wikipedia_use_cases}}, our survey sample is fairly representative in terms of the age distribution. Similar to our sample, the majority of English Wikipedia readers have some amount of college, although the participants who responded to our survey are slightly more skewed towards higher education degrees (PhD).
%\pushkal{How representative is this sample?}

Section 2 (a) is about general particiapnts' engagement with Wikipedia and UK politics. We first asked: \textit{How often do you visit Wikipedia?} % ask how much these participants engage with Wikipedia and the UK Parliament. 
In total 96\% participants visit Wikipedia almost daily or weekly. The remaining 4\% either visit monthly, don't visit or prefer not to say. We then ask how much participants trust Wikipedia on a scale of 1--5 (5 for high trust) we see that 73\% trust Wikipedia either 4/5 or 5/5, similar to previous studies\footnote{\url{https://meta.wikimedia.org/wiki/Research:The_role_of_citations_in_how_readers_evaluate_Wikipedia_articles}}. %21\% of respondents are neutral and only 5\% indicate less trust in Wikipedia. 
Next, we asked participants: \textit{Have you ever read a Wikipedia article on UK MPs?} 74\% replied that they have read at least one MP's Wikipedia article. We then ask participants to express their interest in the UK parliament on the scale 1--5: 30\% responding 5/5 (5 being high interest or knowledge), 14\% indicating 4/5, 26\% 3/5 and the remaining 30\% indicating low knowledge or interest (2/5 or 1/5). %Additionally, 71\% say they have read information about MPs on the search result panel which is curated from Wikipedia (mostly in the top-left panel). Interestingly, 65\% (8\%) say that they mostly (always) click on this panel to open the corresponding Wikipedia page after searching. 

Section 2 (b) has 2 questions with free text answers capturing readers' motivation (\textit{Why do you read MPs pages on Wikipedia?}) and opinion on missing information (\textit{Which  information is missing in the MP Wikipedia Pages you read?}). 

Replies to the first question (motivation) mostly focus on the information need. Participants read UK MPs articles on Wikipedia for general interest; to gather background to news item and controversies; to inspect MPs' personal life and personal details (date of birth etc.); %previous experience/expertise; 
to know more about political views, political activity - voting records etc, and constituency history/information. The structure and content of most MPs' pages appear well-suited to readers who have a general interest or are seeking background information. A typical response to the question on motivation was ``Get basic information about MPs' careers and positions; Get information about political controversies the MP has been involved in''. Figure~\ref{fig:sections} compares the percentage of pages with section categories in relation to overall users' responses about which parts of the pages are most important to them. We see that the Main section is there for almost all pages but only half of the times people are interested in reading it. Based on the responses we see that people are mostly interested in \emph{Political and Parliamentary Career} as well as their \emph{Political views}. Additionally (not shown in figure), almost 15\% say that they read citations on these pages as well.

Only 35\% respondents replied to the second question about missing information. While around 30\% of them finds that no information is missing from Wikipedia articles, others find that pages are missing MPs' voting records and information about MPs' financial interests.  Neither of these information categories are well-represented on the UK Parliament's own website either. At the time of writing, information about MPs' financial interest is not available as machine-readable data\footnote{\url{https://bit.ly/MembersFinancialInterests}} and although an API is available for votes (`Divisions') in both Houses, the information can be hard to understand without considerable research into the context\footnote{\url{https://bit.ly/EnvironmentBil6}}.

\begin{figure}[thb]
    \centering
     \includegraphics[width=0.49\columnwidth]{figures/surveySections.png}
 \caption{
 Section categories in MPs pages and from survey.
}
\end{figure}

\subsection{Discussion}

\textbf{Difficult Readability.}  We find that pages have low readability scores: 98\% of page content has a reading level equivalent to college graduate level, thus making those pages less accessible to people with a lower level of education. This is highly important to fix, as Wikipedia is increasingly the default source of information, and ranks highly in search results for MP names on popular search engines.

\textbf{Alignment with Information Needs.} The survey identifies readers' motivations and draws attention to information which is missing on MPs' pages. We find that, overall, despite difficult readability, readers' information need is well satisfied, and the editing dynamics develop sufficient content coverage. However almost 70\% of readers are interested in reading about political career and political views, although information on the latter topic is less well-represented in the pages.
